# Supplementary material for: Cascaded Sparse Feature Propagation Network for Interactive Segmentation
Source: arXiv:2203.05145 source file (2023-10-30)
Supplement: Supplementary file 1 [file appendix.tex]

\appendix
\section{Datasets}
We evaluate our method over a wide range of datasets including GrabCut, Berkeley, DAVIS, COCO and SBD, by following the standard evaluation protocol.

\textbf{GrabCut\cite{rother2004grabcut}} is a typical interaction segmentation dataset, which contains 50 images with distinguishable foreground and background.

\textbf{Berkeley\cite{mcguinness2010comparative}} contains 96 images with 100 object masks from its test subset.

\textbf{DAVIS\cite{perazzi2016benchmark}} is originally introduced for video segmentation. Only 345 randomly sampled frames with finely labeled objects are used in our method by following \cite{jang2019interactive}.

\textbf{COCO\cite{lin2014microsoft}} is a typical semantic segmentation dataset, containing more complex scene and multiscale objects. Following \cite{xu2016deep}, we split the dataset into COCO(seen) and COCO(unseen) according to their object class whether in PASCAL VOC or not. And finally, 10 images are sampled randomly for each category. For simplicity, we denote COCO(seen) and COCO(unseen) as COCO$^s$ and COCO$^u$

% \textbf{PASCAL VOC\cite{everingham2010pascal}} contains 1449 images with 3427 object masks from its validation set. We ignore evaluating the precision of object boundaries since they are marked.

\textbf{SBD\cite{hariharan2011semantic}} contains 6671 object masks for 2820 images.
\section{More comparison with SAM on iShape Dataset}
To further demonstrate our advantage compared to SAM, we evaluate our model and SAM on the iShape dataset~\cite{yang2021ishape}, which has many thin structure and requires model to segment details. As in Fig.\ref{fig:ishape}, our approach significantly surpass SAM on iShape dataset when number of points exceeds 5, which indicates that out approach is better at segmenting the detailed (slender and long) part. Additionally, as shown in Fig.\ref{fig:ishape_example}, our approach is better at segmenting the detailed (slender and long) parts.
\begin{figure}[!h]
    \centering
    \includegraphics[scale=0.5]{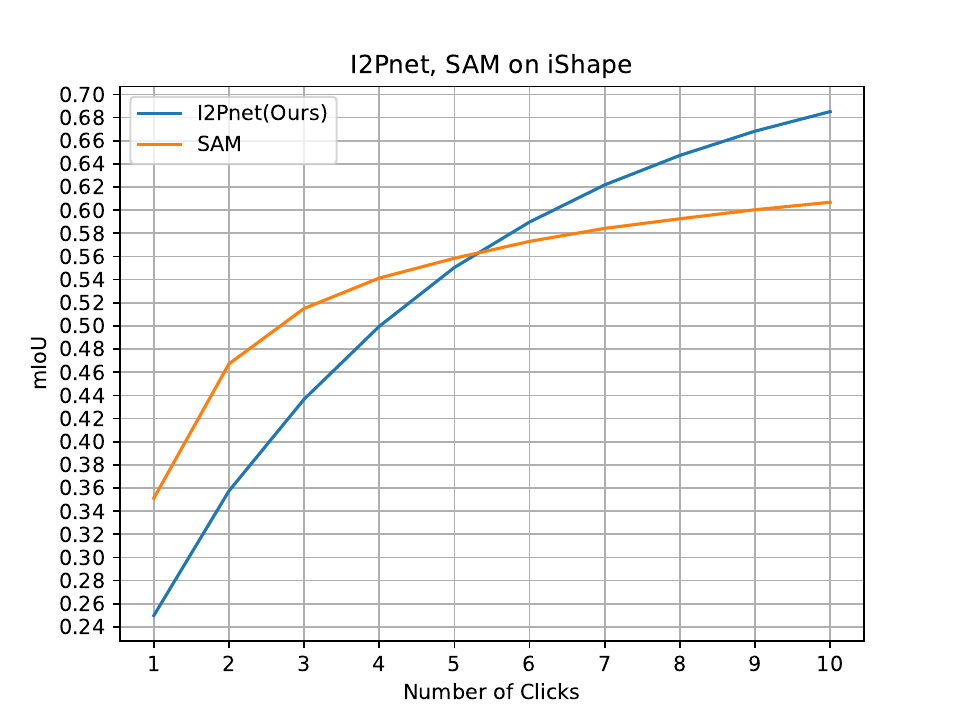}
    \caption{\small{ Comparison with SAM on iShape dataset. It is obvious that although SAM has higher mIoU at first, our I2Pnet quickly catches up and surpass SAM as the number of points increases.}}
    \label{fig:ishape}
\end{figure}
\begin{figure}[!h]
    \centering
    \includegraphics[scale=0.25]{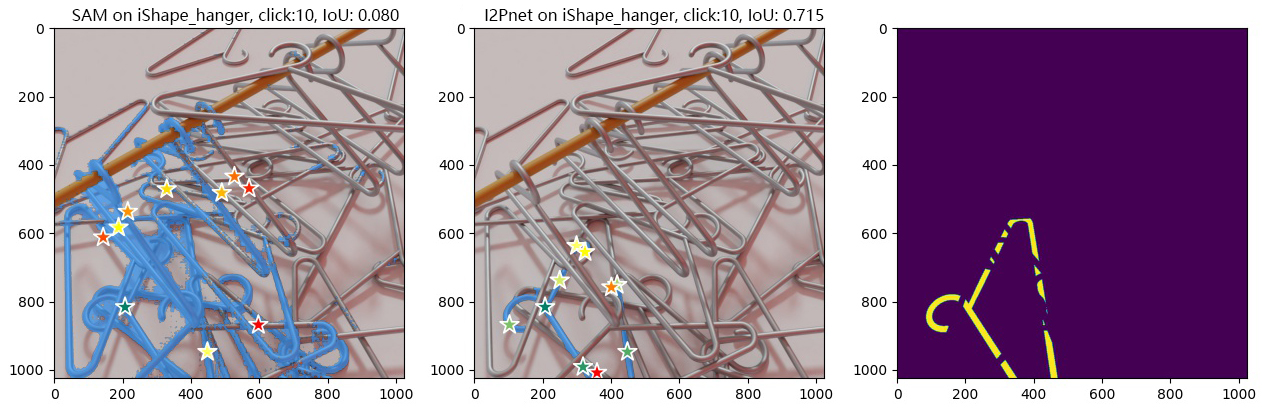}
    \includegraphics[scale=0.25]{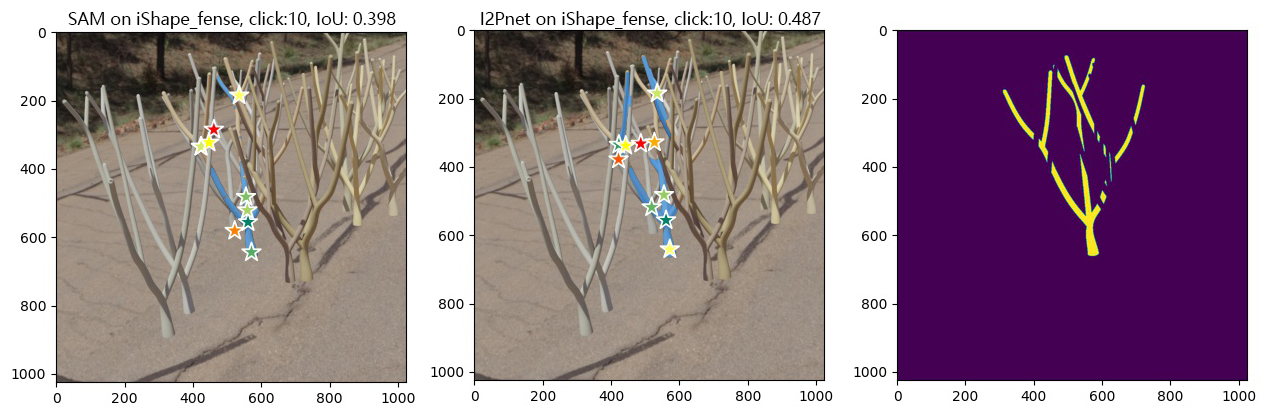}
    \caption{\small{ Examples of comparison with SAM on iShape dataset. They are two examples of "hanger" and "branch" classes in iShape dataset. Points with color from dark green to light green are the positive ones added from early to late, while the ones with color from red to yellow are negative points. The rightmost images are the ground truth. }}
    \label{fig:ishape_example}
\end{figure}

\section{Success samples with different number of clicks}
To further analysis our improvement, we report the distribution of success samples with different number of clicks on the challenging fine-grained DAVIS dataset, which contains 345 samples in total. 
% Compared with previous SOTA RITM~\cite{sofiiuk2021reviving}, 
As in Fig.\ref{fig:barplot}, our approach can successfully segment
71.3\% (246) samples within \textbf{5 clicks}, which greatly outperforms the RITM by 8.1\%. It indicates that we can better utilize user-provided sparse click information.

\section{The performance of boundary}
To validate our design, we utilize cascadePSP to refine the prediction of RITM in each step. We evaluate NoC@90 and boundary IOU when each image is interacted for 20 steps on the challenging DAVIS dataset.
The results in Tab.\ref{b-iou} below show that CascadePSP actually hurts the performance. The main reason is that CascadePSP ignores the human input, which is essential for interactive segmentation. Such smoothing may lead to failure cases when the target region includes multiple object classes, such as segmenting people and horses in Fig.1 (main text). More importantly, compared with FocusCut which refine the boundary progressively, we achieve comparable results on boundary IOU and much lower NoC, illustrating our method can capture user intention and segment the boundary simultaneously.
\begin{figure}[!t]
    \centering
    \includegraphics[scale=0.3]{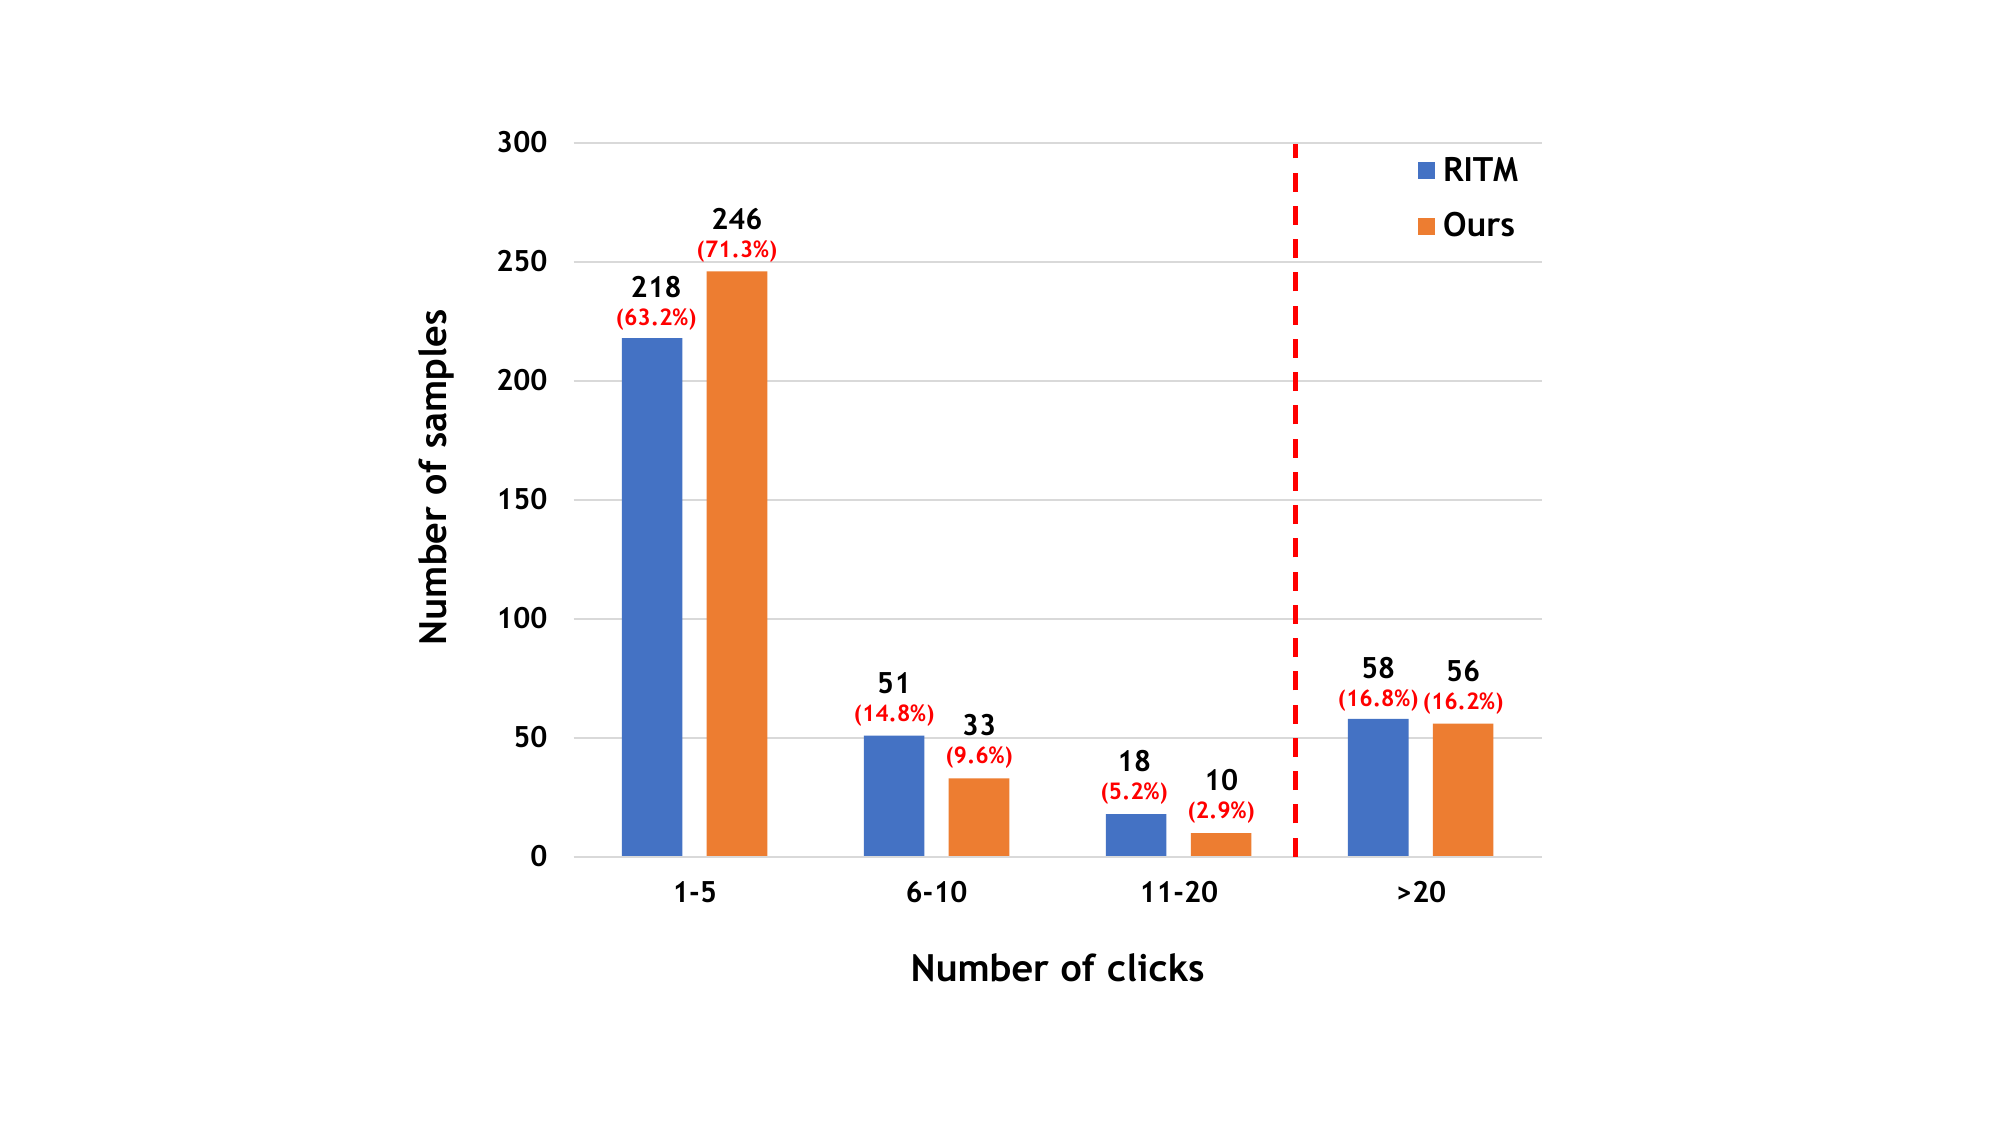}
    \caption{\small{The distribution of the number of clicks on DAVIS dataset. 
    The experiments are on the ResNet-50 backbone. The left of red dotted line is the success samples and the right of 
    red dotted line is the failed samples, which can't reach 90\% IoU within 20 clicks. 
    1-5 means the number of samples that need at least one click and at most five clicks to reach 90\% IoU. }}
    \label{fig:barplot}
\end{figure}
\begin{table}[t]
	\centering 
 	\caption{\small{The performance on DAVIS. Boundary IOU(B-IOU) is evaluated under 20 interactive step.}}
  	\label{b-iou}
	 
	\resizebox{0.6\textwidth}{!}{	
	\begin{tabular}{c|cc}
		\toprule[1pt]
		\textbf{Method} & \textbf{NoC@90} & \textbf{B-IOU(20 steps)} \\ \midrule[0.5pt]
		RITM+CascadePSP & 6.82   & 85.30 \\
		RITM            & 6.68   & 86.25 \\
		FocusCut        & 6.22   & \textbf{87.40} \\
		Ours            & \textbf{5.80}    & 87.07 \\ \bottomrule[1pt]
	\end{tabular}}

\end{table}

\section{HSGN analysis} 
To further investigate the proposed HSGN, we conduct several additional ablations on its design.
As shown in Tab.\ref{HSGN-analysis}, when directly fusing the multi-scale features in HSGN without any sparse
message propagation, the results in 1st \& 2nd row indicate that such design will not bring any performance gain.
Furthermore, we apply another SGN to conduct sparse click message propagation on the high-resolution feature map after fusion. 
The results in 3rd row show that the SGN can propagate annotated click features effectively and benefit the final segmentation results.
However, it still underperforms our proposed HSGN due to its inaccurate affinity calculated on low-level features. Overall, our HSGN performs best compared with
other variants and achieves 6.39 and 5.36 NoC@90 on DAVIS and SBD respectively.

\begin{table}[tp]
    \centering
\caption{\textbf{Ablation study of HSGN on ResNet-34 backbone}. Baseline(BS) is our implementation of RITM\cite{sofiiuk2021reviving}. The Fuse means directly concatenating the high-resolution feature with the high-level feature and then going through a convolution layer with ReLU.}
    \label{HSGN-analysis}

    \resizebox{0.6\textwidth}{!}{
        \begin{tabular}{c|l|ccc}
        \toprule[1pt]
    \textbf{\#} & \textbf{Comparison} &  \textbf{DAVIS} & \textbf{SBD}  \\ \midrule
    1           & BS + SGN                & 6.62           & 5.57          \\
    2           & BS + SGN + Fuse         & 6.75           & 5.51          \\
    3           & BS + SGN + Fuse + SGN   & 6.52           & 5.39          \\
    4           & BS + SGN + HSGN          & \textbf{6.39}  & \textbf{5.36}          \\ \bottomrule[1pt]
    \end{tabular}
    }
    
\end{table}

\section{Undesired annotated point}
We apply random perturbation to the ideal click positions based on a uniform distribution in $[-a,a]^2$. %and we set $a = \{0, 3, 6\}$ pixels.
We re-evaluate RITM and our method on DAVIS under $a = \{0, 3, 6\}$ pixels. %random perturbations of 0, 3 and 6 units. 
The results below indicate that the undesired annotations do cause performance drop. But our method still outperforms the RITM by a large margin and is more robust to the click noises.% less than RITM. % ($5.75 \rightarrow 6.01 \& 6.68\rightarrow 7.15$).
% and outperform the RITM by a large margin.
\begin{table}[t]
	\centering
 	\caption{The results on DAVIS under different perturbations.}
	\label{deviation}
	 
	\resizebox{0.4\textwidth}{!}{	
	\begin{tabular}{c|ccc}
	\toprule[1pt]
	Method	 & $a=0$    & $a=3$    & $a=6$    \\ \midrule[0.5pt]
	RITM & 6.68 & 6.89 & 7.15 \\
	Ours & 5.75 & 5.77 & 6.01 \\ \bottomrule[1pt]
	\end{tabular}}
\end{table}
